# Supplementary material for: Integrating Symbolic Reasoning into Neural Generative Models for Design Generation
Source: arXiv:2310.09383 source file (2024-11-14)
Supplement: Supplementary file 1 [file appendix_gancvx.tex]

\subsection{GAN + CVX Baseline}
\label{sec:gan_cvx}
\FloatBarrier

%\begin{figure}[tbh]
%    \centering
%    \includegraphics[width=\linewidth]{positional_reasoning/figs/glide_cvx_pipeline.png}
%    \caption{GAN + CVX pipeline. \textbf{A)} The full pipeline as a unified system. Three subnetworks are used. A GAN which proposes a list of positions given object data and a constraint list, a pre-trained inpainting model capable of adding the given objects to a background scene, and an adversarial discriminator. \textbf{B)} The architecture of the GAN. \textbf{C)} The inpainting model.}
%    \label{fig:cvxgan}
%\end{figure}

Automated convex optimization is a powerful technique for solving optimization problems where the goal is to find the minimum or maximum value of a given convex function. In this method, a variety of efficient solvers are used to find the optimal solution, as long as all the constraints and the function to be optimized are convex. With recent advancements in the field, these solvers can be easily integrated into neural networks, allowing gradients to propagate through the solver seamlessly.

The GAN + CVX approach relies on this concept. In short, this method is accomplished by creating a GAN which outputs a set of parabolas -- one for each positional variable -- such that the neural net's ``best guess'' for a location is at the vertex. Then the convex optimizer finds the optimal value of the sum of parabolas subject to constraints. If a preferred value is not ruled-out by a constraint, the minimum of that variable's parabola will be selected. If it is ruled out, the result will be as close as possible to it. These constraints must be convex, which limits the library of possible constraints.

%\begin{figure}[tbh]
%    \centering
%    \includegraphics[width=\linewidth]{figs/glide_cvx_pipeline.png}
%    \caption{GAN + CVX pipeline. \textbf{A)} The full pipeline as a unified system. Three subnetworks are used. A GAN which proposes a list of positions given object data and a constraint list, a pre-trained inpainting model capable of adding the given objects to a background scene, and an adversarial discriminator. \textbf{B)} The architecture of the GAN. \textbf{C)} The inpainting model.}
%    \label{fig:cvxgan}
%\end{figure}

\FloatBarrier
